# Supplementary material for: DESIRE: Dynamic Knowledge Consolidation for Rehearsal-Free Continual Learning
Source: arXiv:2411.19154 source file (2024-11-28)
Supplement: Supplementary file 1 [file appendix_stdev.tex]

\begin{table}[h!]
\centering
\caption{Results of SD(ACC) n three datasets under long-phase settings $(T = 10~\text{and}~20)$.}
\begin{tabular}{c!{\vrule width \lightrulewidth}ccccccc} 
\hline
\toprule
         & \multicolumn{2}{c}{\textbf{CIFAR100}} & \multicolumn{2}{c}{\textbf{TinyImageNet}} & \multicolumn{2}{c}{\textbf{ImageNet380}} & \multirow{2}{*}{\textbf{Average}} \\ 
         & 10T & 20T & 10T & 20T & 10T & 20T &  \\
\midrule
LAE-Adapter &
$\text{9.22}$& 
$\text{11.80}$& 
$\text{7.26}$& 
$\text{6.34}$& 
$\text{20.28}$&
$\text{17.16}$& 
$\text{12.01}$   \\
LAE-Prefix &
$\text{6.71}$& 
$\text{10.06}$& 
$\text{8.95}$& 
$\text{7.64}$& 
$\text{9.94}$&
$\text{10.15}$& 
$\text{8.91}$   \\
LAE-LoRA &
$\text{8.39}$& 
$\text{10.35}$& 
$\text{7.40}$& 
$\text{7.00}$& 
$\text{6.21}$&
$\text{7.98}$&
$\text{7.89}$   \\
PASS &
$\underline{4.18}$&
$\underline{5.66}$&
$\underline{3.48}$&
$\underline{5.30}$&
$\textbf{3.14}$&
$\textbf{3.50}$&
$\underline{4.21}$   \\
L2P &
$\text{8.23}$&
$\text{11.07}$&
$\text{7.78}$&
$\text{8.73}$&
$\text{17.87}$&
$\text{17.64}$&
$\text{11.89}$   \\
DualPrompt &
$\text{7.34}$&
$\text{11.58}$&
$\text{6.98}$&
$\text{9.79}$&
$\text{11.31}$&
$\text{6.18}$&
$\text{8.86}$   \\
CODA-Prompt &
$\text{5.41}$&
$\text{10.44}$&
$\text{7.41}$&
$\text{9.22}$&
$\text{5.84}$&
$\text{6.82}$&
$\text{7.52}$   \\
O-LoRA &
$\text{5.18}$&
$\text{11.17}$&
$\text{4.39}$&
$\text{6.96}$&
$\text{4.23}$&
$\text{5.50}$&
$\text{6.24}$   \\
EASE &
$\text{5.81}$&
$\text{10.84}$&
$\text{6.16}$&
$\text{8.20}$&
$\text{6.45}$&
$\text{7.19}$&
$\text{7.45}$   \\
InfLoRA &
$\text{5.19}$&
$\text{12.13}$&
$\text{4.33}$&
$\text{9.15}$&
$\text{3.37}$&
$\text{4.93}$&
$\text{6.52}$   \\
\textbf{Ours} &
$\textbf{4.10}$&
$\textbf{5.59}$&
$\textbf{3.06}$&
$\textbf{5.00}$&
$\underline{3.25}$&
$\underline{3.65}$&
$\textbf{4.11}$   \\
\Xhline{3.5\arrayrulewidth}
\end{tabular}
\label{tab:appendix_stdev}
\vspace{-8pt}
\end{table}
